# Supplementary material for: Enhanced Sensitivity to Blackbody Radiation in Spintronic Poisson Bolometers
Source: arXiv:2512.12490 ancillary file (2026-09-04)
Supplement: Supplementary file 1 [file Supplementary_Long_Wave_Infrared_Spintronic_Poisson_Bolometers_with_High_Sensitivity.pdf]

# Supplemental Information for Long-Wave Infrared Spintronic Poisson Bolometers with High Sensitivity

Ziyi Yang, Sakshi Gupta, Jehan Shalabi, Daien He, Leif Bauer, Angshuman Deka, Zubin Jacob\*

Ziyi Yang, Jehan Shalabi, Dr. Daien He, Dr. Leif Bauer, Prof. Zubin Jacob

Elmore Family School of Electrical and Computer Engineering, Purdue University, West Lafayette, Indiana 47907, USA

Sakshi Gupta

Department of Physics and Astronomy, Purdue University, West Lafayette, Indiana 47907, USA

Dr. Angshuman Deka

Birck Nanotechnology Center, Purdue University, West Lafayette, Indiana 47907, USA

Email Address: zjacob@purdue.edu

## 1 Magnetic Tunnel Junction (MTJ) Layer Stack

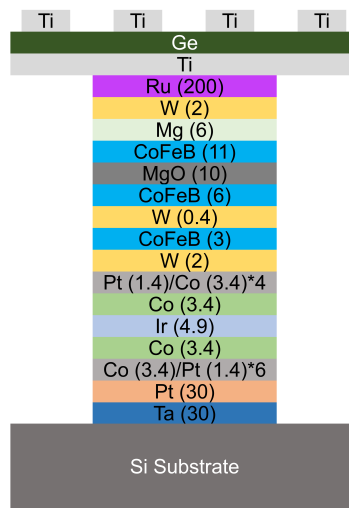

Figure 1: Layer stack of the magnetic tunnel junction. The numbers represent thicknesses in angstroms.

## 2 Simulation of the Plasmonic Absorber

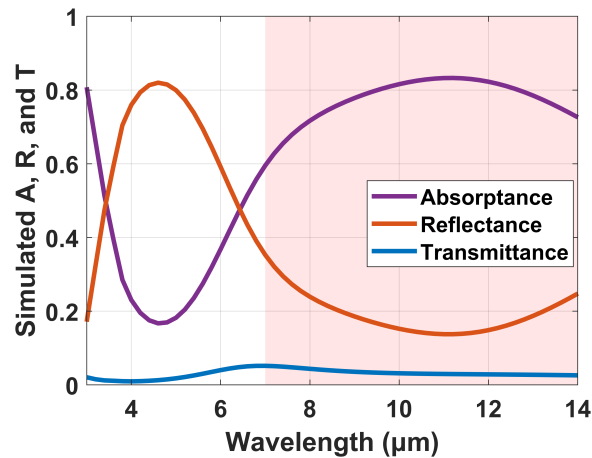

Figure 2: Simulated absorptance, reflectance, and transmittance of the broadband LWIR plasmonic absorber.

Table 1: Sensing Layer Temperature Increase with Different Plasmonic Absorbers

| Blackbody temperature | Absorber in [1] | This paper |
|-----------------------|-----------------|------------|
| 298.15 K              | 130.9 mK        | 501.5 mK   |
| 303.15 K              | 143.1 mK        | 548.6 mK   |

Compared to the broadband MWIR plasmonic absorber design in [1], the broadband LWIR plasmonic absorber in this paper enables around 4 times the original temperature increase in the sensing layer according to the heat transfer simulation by COMSOL.

### 3 Experimental Setup

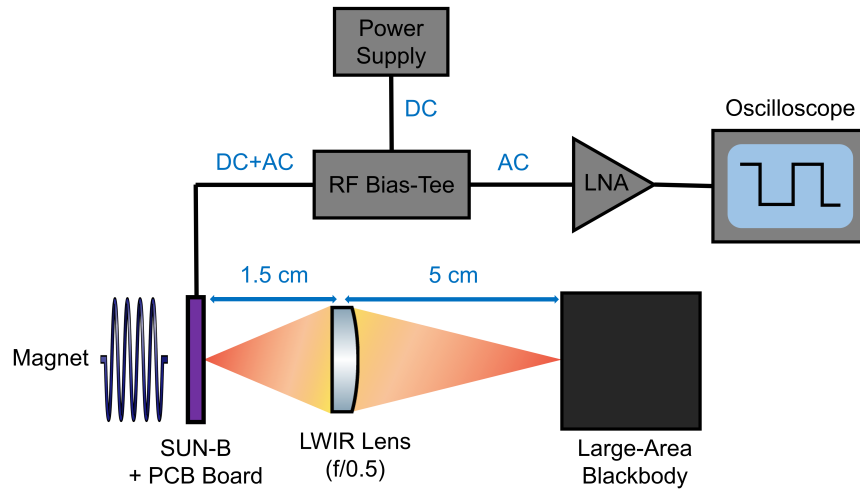

Figure 3: Experimental Setup. Power Supply: applies bias voltage to the SUN bolometer. RF Bias-Tee: bandwidth 4 kHz-40 GHz. DC bias voltage is applied to the SUN bolometer, and the AC component of the response is directed to the oscilloscope for readout. LNA: 31 dB broadband low-noise amplifier (9 kHz-3 GHz). Oscilloscope: DC-4 GHz; Maximum sampling rate is 20 GHz.

### References

- [1] L. Bauer, A. Deka, M. A. Mousa, S. Gupta, D. He, S. Huang, B. Prasad, T. Santos, B. Ray, Z. Jacob, *Nano Letters* **2025**, *25*, 14 5599.
